# Supplementary material for: Meta-validation of bipartite network projections
Source: arXiv:2105.03391 source file (2022-04-05)
Supplement: Supplementary file 1 [file SI.pdf]

# Meta-validation of bipartite network projections: Supplementary Information

Giulio Cimini,[1,2] Alessandro Carra,[3] Luca Didomenicantonio,[3] and Andrea Zaccaria[4,2]

[1] *Physics Department and INFN, University of Rome Tor Vergata, 00133 Rome (Italy)*
[2] *Enrico Fermi Research Center, 00184 Rome (Italy)*
[3] *Physics Department, Sapienza University of Rome, 00185 Rome (Italy)*
[4] *Institute for Complex Systems (CNR) UoS Sapienza, 00185 Rome (Italy)*

## SUPPLEMENTARY NOTE 1: RIGHT VS LEFT TAIL TEST OF STATISTICAL SIGNIFICANCE

The definition of p-value – same of eq. (3) of the main text

$$p[C_{ij}] = 1 - \sum_{x=0}^{C_{ij}-1} \pi(x|i,j), \tag{S1}$$

is the probability that $i$ and $j$ have no less than $C_{ij}$ co-occurrences in the null model [1]. This definition plus the condition of statistical significance $p[C_{ij}] < p^*$ is useful to detect the co-occurrences that are significantly *larger* than their null model expectations. We use such a one-tailed test (the right tail one) because we associate a significantly large value of co-occurrences to a signal of real interdependence between the two nodes involved. Hence, we are not interested in detecting the empirical co-occurrences that are significantly *smaller* than the null model expectations.

Nevertheless, it is straightforward to implement the left tail test as well, by defining the p-value as

$$p'[C_{ij}] = \sum_{x=0}^{C_{ij}} \pi(x|i,j), \tag{S3}$$

plus the same condition of statistical significance $p[C_{ij}] < p^*$. The right-hand side of eq. (S3) is now the probability that $i$ and $j$ have no more than $C_{ij}$ co-occurrences in the null model. Differently from the right tail test, however, it

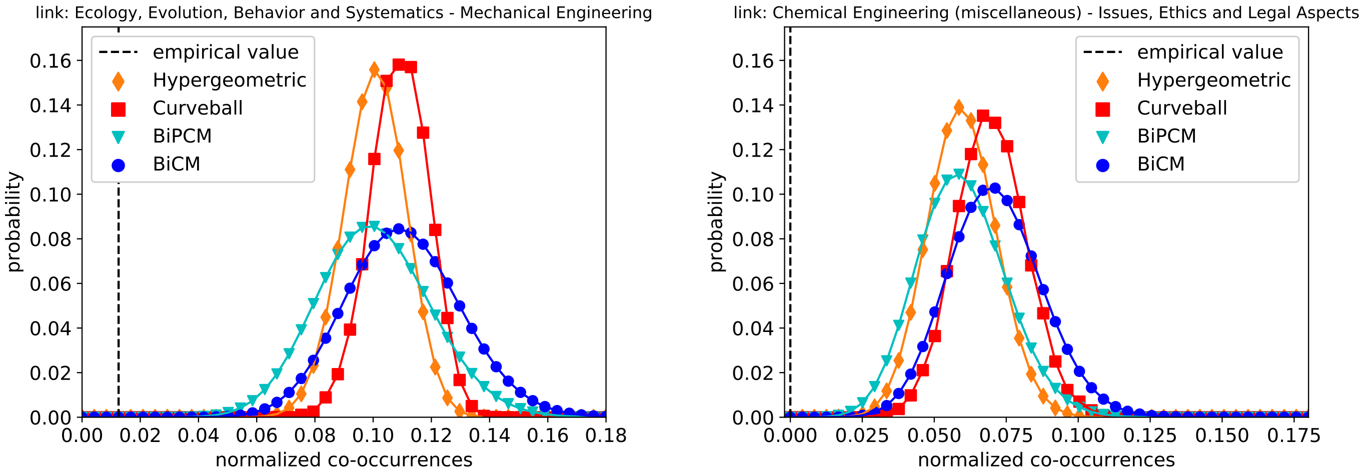


Supplementary Figure 1. Comparison of empirical co-occurrences and their null model distributions for representative scientific field pairs. (left) *Ecology, Evolution, Behavior and Systematics - Mechanical Engineering*, (right) *Chemical Engineering (miscellaneous) - Issues, Ethics and Legal Aspects*. For each pair $(i, j)$ of scientific fields we report the empirical value of the (normalized) co-occurrences $C_{ij}/|\Gamma|$ and the respective null model distributions $\pi(\cdot|i,j)$. For the left tail test, the p-value is given by the area under the distribution up to the empirical value.

[1] Note that co-occurrences $C_{ij}$ are a discrete variable, therefore the null model distribution $\pi(\cdot|i,j)$ has a discrete support ranging from 0 to $\min[k_i, k_j]$. The p-value definition of eq. (S1) commonly used in the literature is the sum of $\pi(\cdot|i,j)$ starting from the empirical value of $C_{ij}$ included. The other possibility would be to exclude $C_{ij}$ from the sum domain, resulting in

$$p[C_{ij}] = 1 - \sum_{x=0}^{C_{ij}} \pi(x|i,j). \tag{S2}$$

The two approaches would coincide if $C_{ij}$ were a continuous variable. In our discrete case, we checked that they lead to almost identical results, after a proper re-scaling of the significance threshold $p^*$.

is less clear what kind of signal can be associated to the co-occurrences that pass such statistical test. Supplementary Figure 1 shows two example of significantly small co-occurrences between pairs of scientific fields, which appear quite unrelated to each other.

Overall, as shown in Supplementary Figure 2, the number of link validated by the right tail test (panel A – which is the same of Figure 4 in the main text) is typically higher than the number of links validated by the left tail test (panel B), especially for partial models (this happens due to the relative position of the mean between partial and full models). This observation confirms that empirical data on the scientific activity of country is biased towards the right tail and that therefore there is a non-trivial signal of interdependence and common capability requirements between scientific fields.

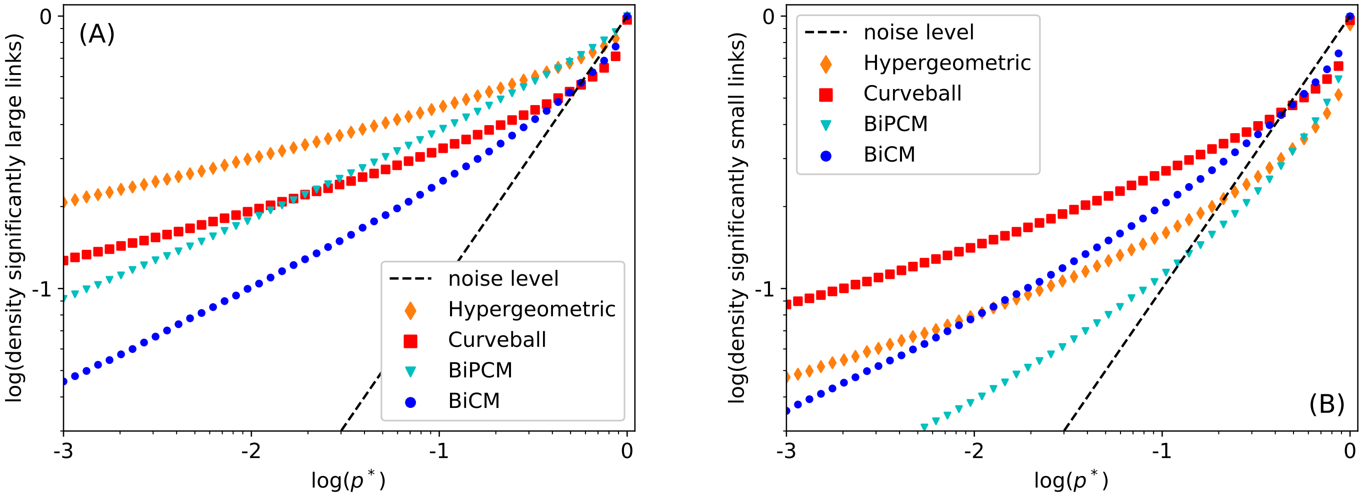


Supplementary Figure 2. Density $\rho$ of links validated by the various null models as a function of the significance threshold $p^*$. Panels (A) and (B) report results of the right / left tail test, which validates the links that are significantly larger / smaller than the null model expectations, respectively.

## SUPPLEMENTARY NOTE 2: NULL MODELS OF WEIGHTED MONOPARTITE NETWORKS

As discussed in the main text, the task of filtering a bipartite network projection can be in principle accomplished using a null model defined directly on the projection, instead of a null model defined on the original bipartite network. Since the projection of a bipartite network is a (dense) weighted monopartite network, we can use a null model formulation that constraints the strength sequence of the projection, where the strength of generic node $i$ is given by $s_i = \sum_{j(\neq i)\in \mathrm{L}} C_{ij}$. Here we consider two popular model formulations.

### Disparity Filter

The *Disparity Filter* [1] relies on the null hypothesis that node $i$ distributes its total strength $s_i$ in a uniform random division among its neighbors. If we denote by $d_i$ the degree of node $i$ in the projected network (*i.e.*, $d_i = \sum_{j(\neq i)\in \mathrm{L}} \Theta[C_{ij}]$ where $\Theta[x] = 1$ if $x > 0$ and $\Theta[x] = 0$ otherwise), the corresponding null model distribution can be expressed as

$$\pi(x|i,j) = \frac{d_i - 1}{s_i}\left(1 - \frac{x}{s_i}\right)^{d_i - 2} \tag{S4}$$

This expression is obtained by considering $d_i - 1$ points distributed with uniform probability in the interval $[0, s_i]$. These points divide this interval into $d_i$ sub-intervals, whose lengths represent the expected values for the $d_i$ weights according to the null hypothesis. Note that differently from the models discussed in the main text, eq. (S4) is not symmetric in $i, j$ and indeed depends only on node $i$'s properties. Therefore we assign a p-value to the link $i, j$ by averaging the p-values obtained by testing the link from both the perspectives of node $i$ and of node $j$, that is, $p[C_{ij}] = 1 - \frac{1}{2}\sum_{x=0}^{C_{ij}-1}[\pi(x|i,j) + \pi(x|j,i)]$.

### Weighted Configuration Model

The maximum-entropy model that constraints the ensemble average of nodes strength sequence is known as *Weighted Configuration Model* (WCM) [2, 3]. The WCM Hamiltonian is $H(\tilde{\mathbf{C}}, \{\eta_i\}) = \sum_{i\in \mathrm{L}} \eta_i s_i(\tilde{\mathbf{C}})$ where $\{\eta_i\}$ is the set of Lagrange multipliers associated to the constraints $\{s_i\}$. Also in this case the partition function can be computed analytically and the ensemble probability factorizes into link-specific terms, each of which is simply the probability distribution of the co-occurrences:

$$\pi(x|i,j) = q_{ij}^x(1 - q_{ij}). \tag{S5}$$

This is a geometric distribution with success probability $q_{ij} = e^{-\eta_i - \eta_j}$ and expected value

$$\langle C_{ij}\rangle = \frac{q_{ij}}{1 - q_{ij}}. \tag{S6}$$

Finally the numerical values of the Lagrange multipliers are determined by maximising the likelihood of the empirical projected network $\mathbf{C}$ in the ensemble, which implies solving the constraints equations $s_i = \sum_{j(\neq i)\in \mathrm{L}} q_{ij}/(1 - q_{ij})\ \forall i$.

### Comparative analysis of validation outcomes

Supplementary Figures 3 and 5 show that the null model distributions for Disparity Filter and WCM feature an extreme positive skewness but also a much longer tail than the bipartite models counterparts. The effect is that they end up validating nothing also for very large significance thresholds $p^*$. Therefore the information on the bipartite network that originated the projection (which these two models discard) is essential to extract significant information on the projection itself. At last, Supplementary Figure 4 shows that Disparity Filter behaves approximately as a microcanonical model when compared to the canonical WCM.

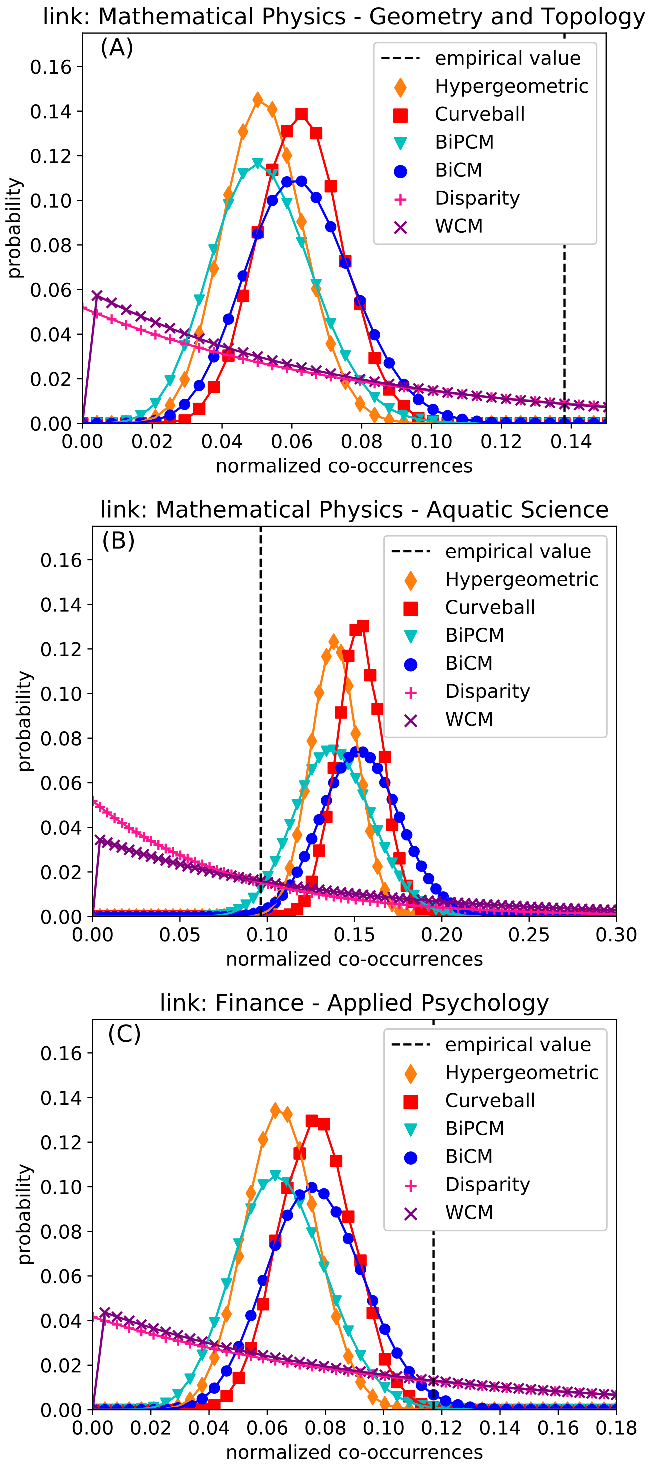


Supplementary Figure 3. Comparison of empirical co-occurrences and their null model distributions for representative scientific field pairs. (A) *Mathematical Physics - Geometry and Topology*, (B) *Mathematical Physics - Aquatic Science*, (C) *Finance - Applied Psychology*. For each pair $(i, j)$ of scientific field we report the empirical value of the (normalized) co-occurrences $C_{ij}/|\Gamma|$ and the respective null model distributions $\pi(\cdot|i, j)$. model distributions $\pi(\cdot|i, j)$. This figure is the same of Figure 2 of the main text with the addition of Disparity Filter and WCM.

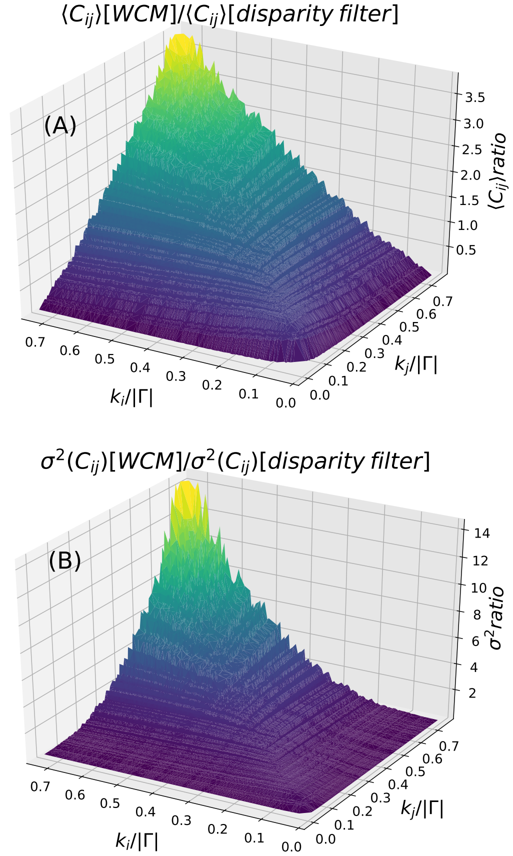


Supplementary Figure 4. Comparison of null model features. (A) Ratio of average co-occurrences $\langle C_{ij}\rangle$ and (B) ratio of variances $\sigma^2(C_{ij})$ for WCM and Disparity Filter, as a function of the normalized degrees $k_i/|\Gamma|$ and $k_j/|\Gamma|$ of the corresponding nodes.

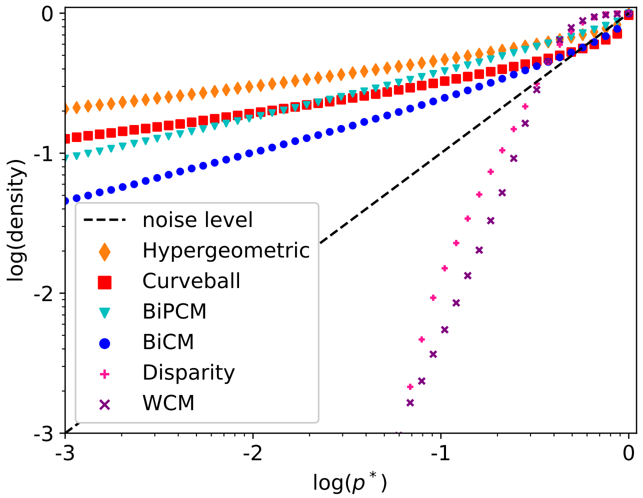


Supplementary Figure 5. Density $\rho$ of links validated by the various null models as a function of the significance threshold $p^*$. The dashed bisector denotes the noise level, namely the probability to statistically validate a null model event. This figure is the same of Figure 4 of the main text with the addition of Disparity Filter and WCM.

## SUPPLEMENTARY NOTE 3: TOTAL CO-OCCURRENCES

Further insights on the features of the various null model formulations can be gained by studying the distribution of the total co-occurrences

$$S = \sum_{\{i,j\}\in \mathrm{L}} \langle C_{ij} \rangle. \tag{S7}$$

In agreement with the discussion in the main text, Supplementary Figure 6 shows that these distributions behave very differently for the various null models. The mean of the two partial models (Hypergeometric and BiPCM) coincide, as well as the mean of the two full models (Curveball and BiCM), with the former smaller than the latter. Moreover, microcanonical models (Hypergeometric and Curveball) feature a Dirac delta distribution because of the hardness of imposed constraints. This can be seen by noting that $S \equiv \sum_{\alpha\in\Gamma} \langle k_\alpha \rangle^2$, a number which is fixed in both microcanonical ensembles. Canonical models (BiPCM and BiCM) instead feature a similar (finite) standard deviation, very small in comparison with the difference of means so that the respective distribution do not overlap.

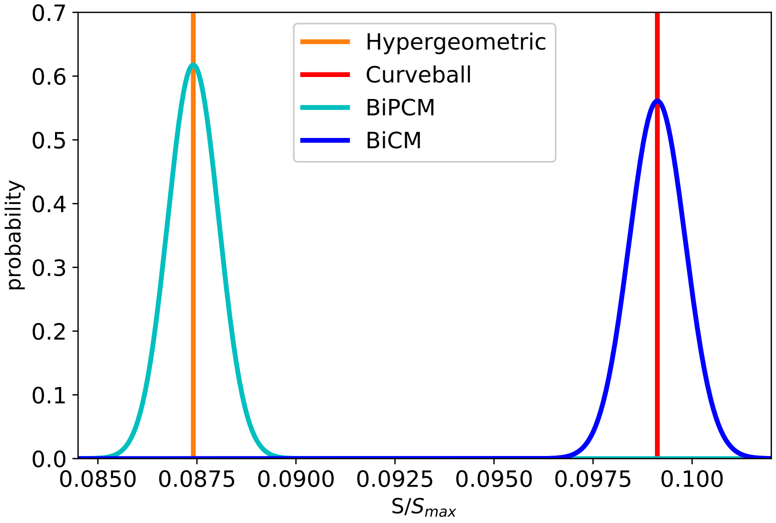


Supplementary Figure 6. Probability distribution of the total co-occurrences $S$ (normalized by their maximum value $S_{max} = |L|^2|\Gamma|$ of a fully connected bipartite network) in the various null model formulations.

## SUPPLEMENTARY NOTE 4: CORRECTION FOR MULTIPLE TESTING WITH THE FALSE DISCOVERY RATE

The statistical hypothesis testing procedure described in the main text applies the same significance threshold or confidence level $p^*$ to each test considered individually. Then we vary $p^*$ to compare the various null model outcomes. However we can also consider a correction for $p^*$ in order to obtain a confidence level for the whole family of simultaneous tests. This is a common approach in the literature to minimize Type I errors; in the context of bipartite network projections, it can be appropriate when co-occurrences between the various node pairs cannot be considered independent realization of a generative process (however they still represent different instances).

Here we study whether this correction would have similar effects for the various null models. This is trivially true for the Bonferroni correction, which simply consists in rescaling the threshold $p^*$ by the number of hypothesis tested, namely $m = \mathrm{L}(\mathrm{L}-1)/2$ (the same number for all null models). The same outcome is not guaranteed for the False Discovery Rate (FDR) [4], which for a given $p^*$ prescribes to order the observed p-values in ascending order (denoting them by $p^{(1)}, \dots, p^{(m)}$) and validate the $k$ smallest p-values, where $k$ is such that $p^{(k)} \leq kp^*/m$.

Supplementary Figure 7 shows that FDR reduces the number of links that are validated in a similar fashion among the various null models: we do not observe a situation in which the correction is minimal for a null model while for another is more pronounced. Therefore we can conclude that correcting for multiple tests causes a rescaling of the validated network density with respect to $p^*$, but does not alter qualitatively the results of our analysis.

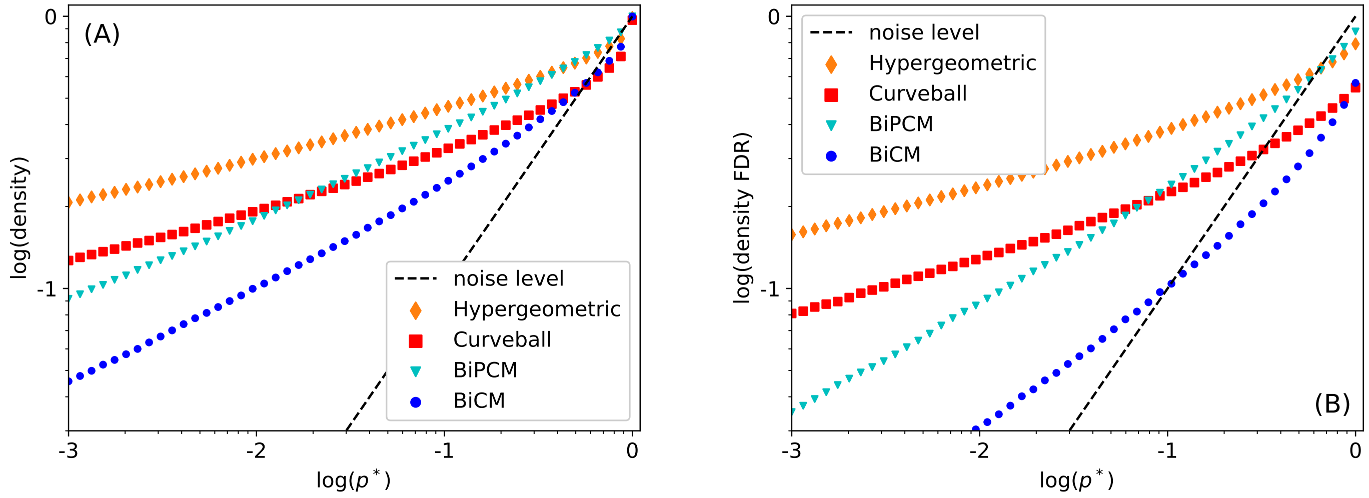


Supplementary Figure 7. Density $\rho$ of links validated by the various null models as a function of the significance threshold $p^*$, with no correction for multiple tests (panel A) and correction with False Discovery Rate (panel B) applied to all null models.

## SUPPLEMENTARY NOTE 5: COMMUNITY DETECTION WITH BAYESIAN STOCHASTIC BLOCKMODELING

In this section we check the consistency of our results using a community detection method based on Bayesian inference of the best stochastic blockmodel (SBM) fit of the network [5, 6]. The cost function to minimize in this case is called *description length*, which represents the amount of information needed to describe the network. A detailed description of the method and the accompanying code is available at `https://graph-tool.skewed.de/static/doc/demos/inference/inference.html#the-stochastic-block-model-sbm`.

Supplementary Figures 8-10 show that this method leads to a rather different network partition characterized by many more communities. Obtaining different outcomes is common when there is no clear-cut community structure, which is typically the case with empirical applications. However the main point of our work, namely that the various null models can lead to a shared community structure, and that in order to find such meta-structure the validated networks should be compared at identical density values, is still supported by these results.

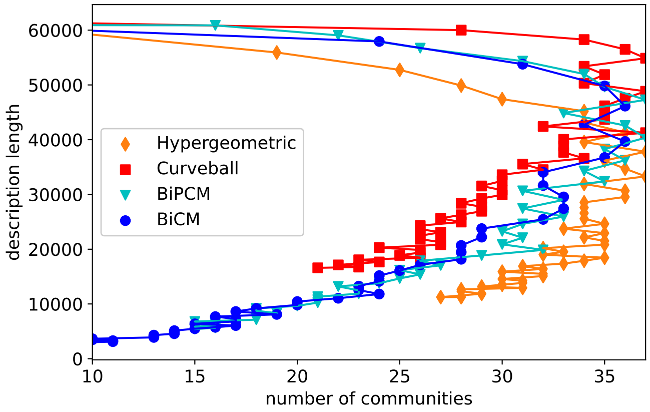


Supplementary Figure 8. Description length versus number of communities for the best SBM partition obtained on the network validated using the various null models. As in the case of Modularity, also here the curves of the various models collapse onto each other.

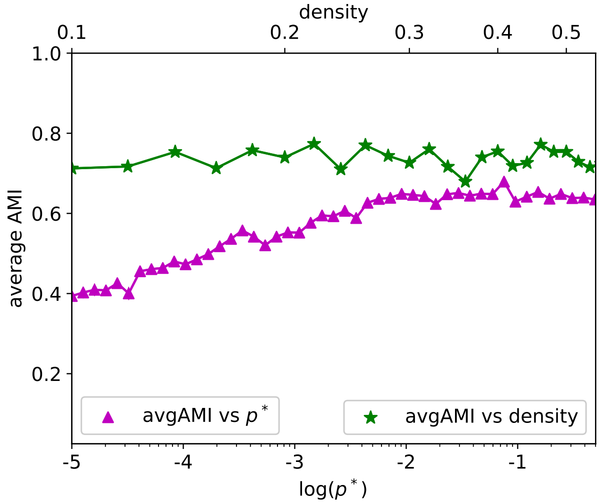


Supplementary Figure 9. Average AMI between the best SBM partitions of the network validated by the various null models. Values are plotted for filtered networks obtained with the same $p^*$ (magenta triangles) or of equal density (green stars). The latter option reveals a higher concordance among the null models.

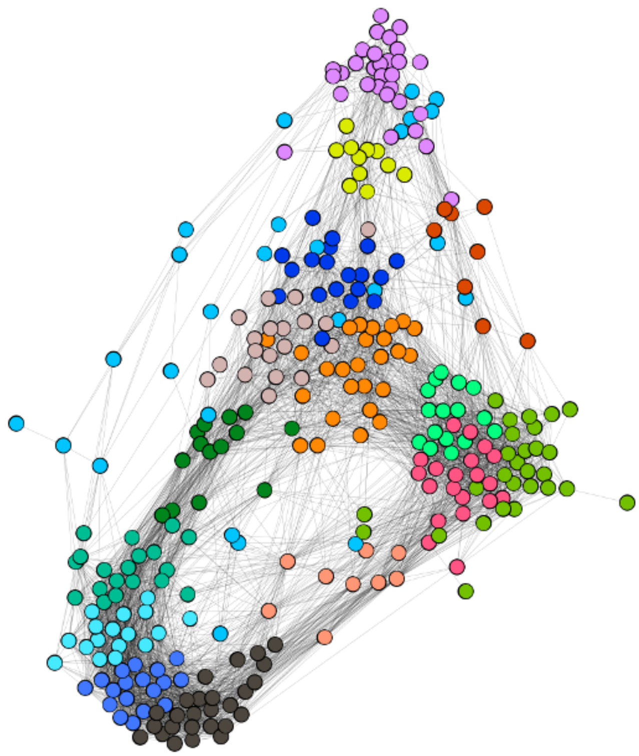

Supplementary Figure 10. SBM-induced community structure for the network of co-occurrence between scientific fields, validated by the BiCM null model for $p^* = 0.0126$ and $\rho = 0.18$ (corresponding to the maximum AMI as of Supplementary Figure 9).

## SUPPLEMENTARY NOTE 6: TEST ON BIPARTITE NETWORKS FROM DIFFERENT DOMAINS

To further support the general applicability of our framework, here we report results of the same analysis performed in the main text for several other bipartite networks belonging to totally different contexts [2]. The purpose is to show that our framework can be generalized when the nature of both nodes and links change drastically. We consider:

- *HOST-VIRUS*: a network of 586 viruses, 754 mammalian species, and 2805 relations between mammalians and viruses they can host (*i.e.*, be infected by) [7]. We consider co-occurrences between mammalians, defined in terms of number of different viruses they can both host. Data available at `https://github.com/cjcarlson/brevity/tree/master/Olival%20Nature%202017%20Raw%20Data`. Results are reported in Supplementary Figure 13.
- *ROBERT* plant: a network of 1429 animal species visiting flowers of 456 plant species that grew in a small area in southwestern Illinois, USA [8]. We consider co-occurrences between plant species, defined in terms of the different animal species they are visited by. Data available at `https://iwdb.nceas.ucsb.edu/html/robertson_1929.html`. Results are reported in Supplementary Figure 14.
- *TAYLOR* World Cities: a network about the service values (indicating the importance of a city in the office network of a firm) of 100 global service firms distributed across 315 cities worldwide [9]. Data are collected in year 2000; links are weighted according to the service value, ranging from 0 to 5. We thus employed the RCA filter and consider co-occurrences between cities, defined in terms of the different important firms office they host in common. Data available at `http://vlado.fmf.uni-lj.si/pub/networks/data/mix/mixed.htm`. Results are reported in Supplementary Figure 15.
- *DUTCH* elite: a network of 200 persons (corporate elite) who sit on the boards of the 395 most important administrative bodies in The Netherlands [10]. We consider co-occurrences between corporate elites, defined in terms of the different boards they both sit on. Data available at `http://vlado.fmf.uni-lj.si/pub/networks/data/2mode/DutchElite.htm`. Results are reported in Supplementary Figure 16.
- *CRIME*: network of 829 persons and 551 crime cases (collected in 1990s in St. Louis), with link connecting persons to the cases where they appeared as either a suspect, a victim, a witness. We consider co-occurrences between crimes, defined in terms of persons appearing in both. Data available at `http://konect.cc/networks/moreno_crime/`. Results are reported in Supplementary Figure 17.
- *MOVIELENS*: a network of 1000 users, 1700 movies, and 100000 ratings from users to movies [11] (we consider as actual links only the ratings bigger than 3). We consider co-occurrences between movies, defined in terms of number of different users that rated both of them. Data available at `https://grouplens.org/datasets/movielens/100k/`. Results are reported in Supplementary Figure 18.

Despite the different nature of these networks, in general we find the same results of the analysis in the main text, namely that the equal-density criterion reveals a consistently higher concordance among the null models. In particular, concerning the community structure, often we can identify a region of "best" agreement between the validation models, indicating which density value (and, as a consequence, which $p^*$) should be chosen in order to obtain a meta-validated network. This happens when we can find a sufficiently high value of modularity, *i.e.*, when a robust community structure emerges — as in the case of HOST-VIRUS (Supplementary Figure 11, where we also compare with metadata-induced partitions) as well as for other networks (Supplementary Figure 12). Otherwise, as in the case of MOVIELENS, the AMI values obtained at equal density are not too far from the values obtained at equal $p^*$, signaling the absence of a community structure in the network.

---

[2] Note that we are limited in the choice of dataset that we can use for our exercise for a twofold reason. Firstly, we need a bipartite network with a meaningful modular projection and possibly with metadata. Secondly, in order to include the Curveball algorithm (that relies on numerical sampling) we cannot consider very large systems.

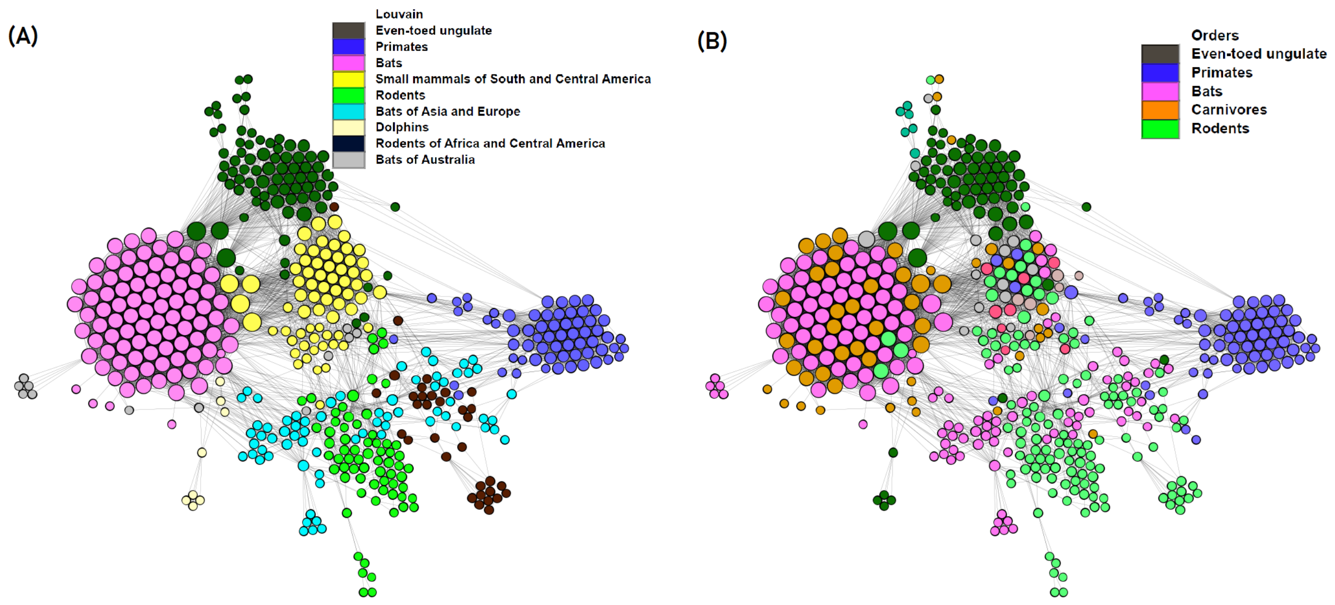


Supplementary Figure 11. *HOST-VIRUS* network: (A) Community structure of the network of co-occurrence between mammalian species (with co-occurrences defined in terms of viruses they can both host), validated by the Hypergeometric null model for $\rho = 0.057$ corresponding to maximum AMI value of the bottom right panel in Supplementary Figure 13. Each color identifies a community (hand-labeled by us as in the legend) shared among the four validated networks. (B) As a comparison, we report the same network with mammalian species labeled according to their species order.


[1] M. A. Serrano, M. Boguñá, and A. Vespignani, Extracting the multiscale backbone of complex weighted networks, PNAS **106**, 6483 (2009).

[2] D. Garlaschelli and M. I. Loffredo, Generalized bose-fermi statistics and structural correlations in weighted networks, Physical Review Letters **102**, 038701 (2009).

[3] T. Squartini and D. Garlaschelli, Analytical maximum-likelihood method to detect patterns in real networks, New Journal of Physics **13**, 083001 (2011).

[4] Y. Benjamini and Y. Hochberg, Controlling the false discovery rate: A practical and powerful approach to multiple testing, Journal of the Royal Statistical Society. Series B (Methodological) **57**, 289 (1995).

[5] T. P. Peixoto, Efficient monte carlo and greedy heuristic for the inference of stochastic block models, Physical Review E **89**, 012804 (2014).

[6] T. P. Peixoto, Bayesian stochastic blockmodeling, in *Advances in Network Clustering and Blockmodeling* (John Wiley & Sons, Ltd, 2019) Chap. 11, pp. 289–332.

[7] K. J. Olival, P. R. Hosseini, C. Zambrana-Torrelio, N. Ross, T. L. Bogich, and P. Daszak, Host and viral traits predict zoonotic spillover from mammals, Nature **546**, 646 (2017).

[8] C. Robertson, *Flowers and insects: lists of visitors of four hundred and fifty-three flowers* (Carlinville, Ill., 1977).

[9] P. Taylor and B. Derudder, *World City Betwork: A Global Urban Analysis* (Routledge, 2015).

[10] W. de Nooy, Ringen om de macht, in *De elite. De Volkskrant Top 200 van invloedrijkste Nederlanders*, edited by W. Dekker and B. Raaij (Amsterdam, The Netherlands: Meulenhoff, 2006) pp. 85–94.

[11] F. M. Harper and J. A. Konstan, The movielens datasets: History and context, ACM Transactions on Interactive Intelligent Systems **5**, 1 (2015).

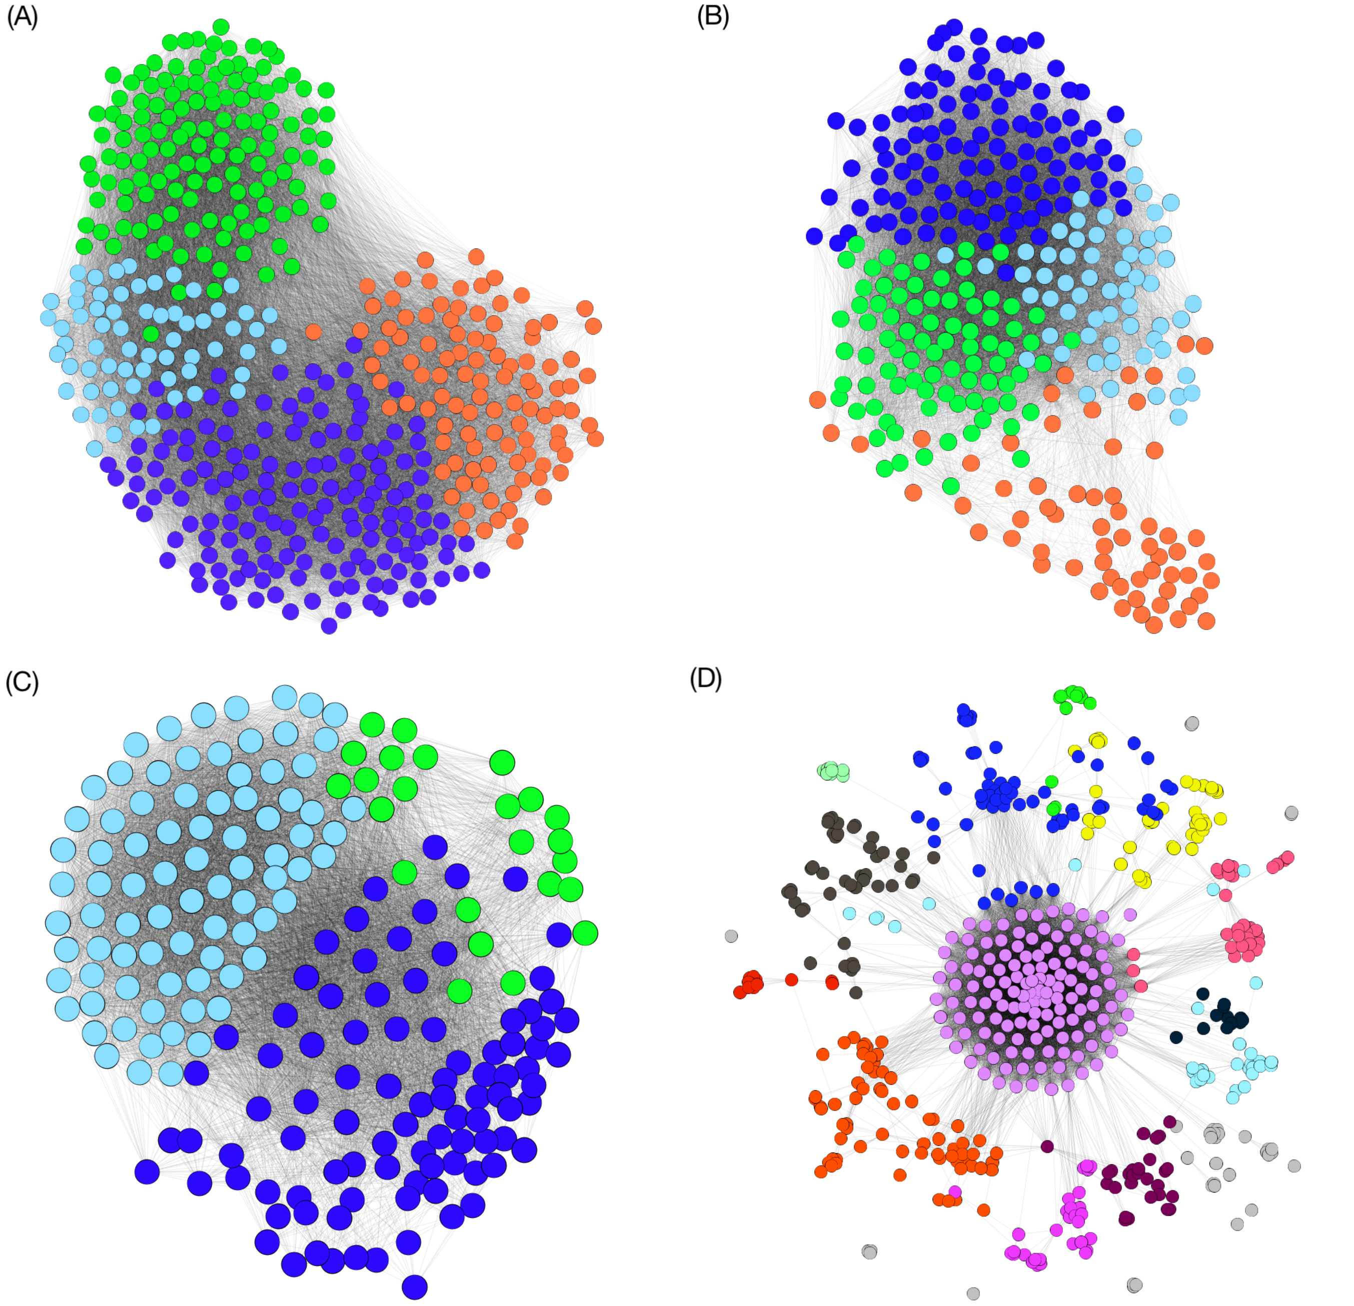


Supplementary Figure 12. Community structures of other networks in our dataset validated by the BiCM null model. Each color identifies a community shared among the four validated networks. (A) *ROBERT* network of co-occurrence between plant species, defined in terms of animal species they are visited by, for $\rho = 0.29$ corresponding to maximum AMI as of Supplementary Figure 14, bottom right panel. (B) *TAYLOR* network of co-occurrence between cities, defined in terms of the different large firms office they host in common, for $\rho = 0.36$ corresponding to maximum AMI as of Supplementary Figure 15, bottom right panel. (C) *DUTCH* network of co-occurrence between corporate elites, defined in terms of the different boards they both sit on, for $\rho = 0.43$ corresponding to maximum AMI as of Supplementary Figure 16, bottom right panel. (D) *CRIME* network of co-occurrence between persons, defined in terms of the different cases they appeared in, for $\rho = 0.08$ corresponding to maximum AMI as of Supplementary Figure 17, bottom right panel.

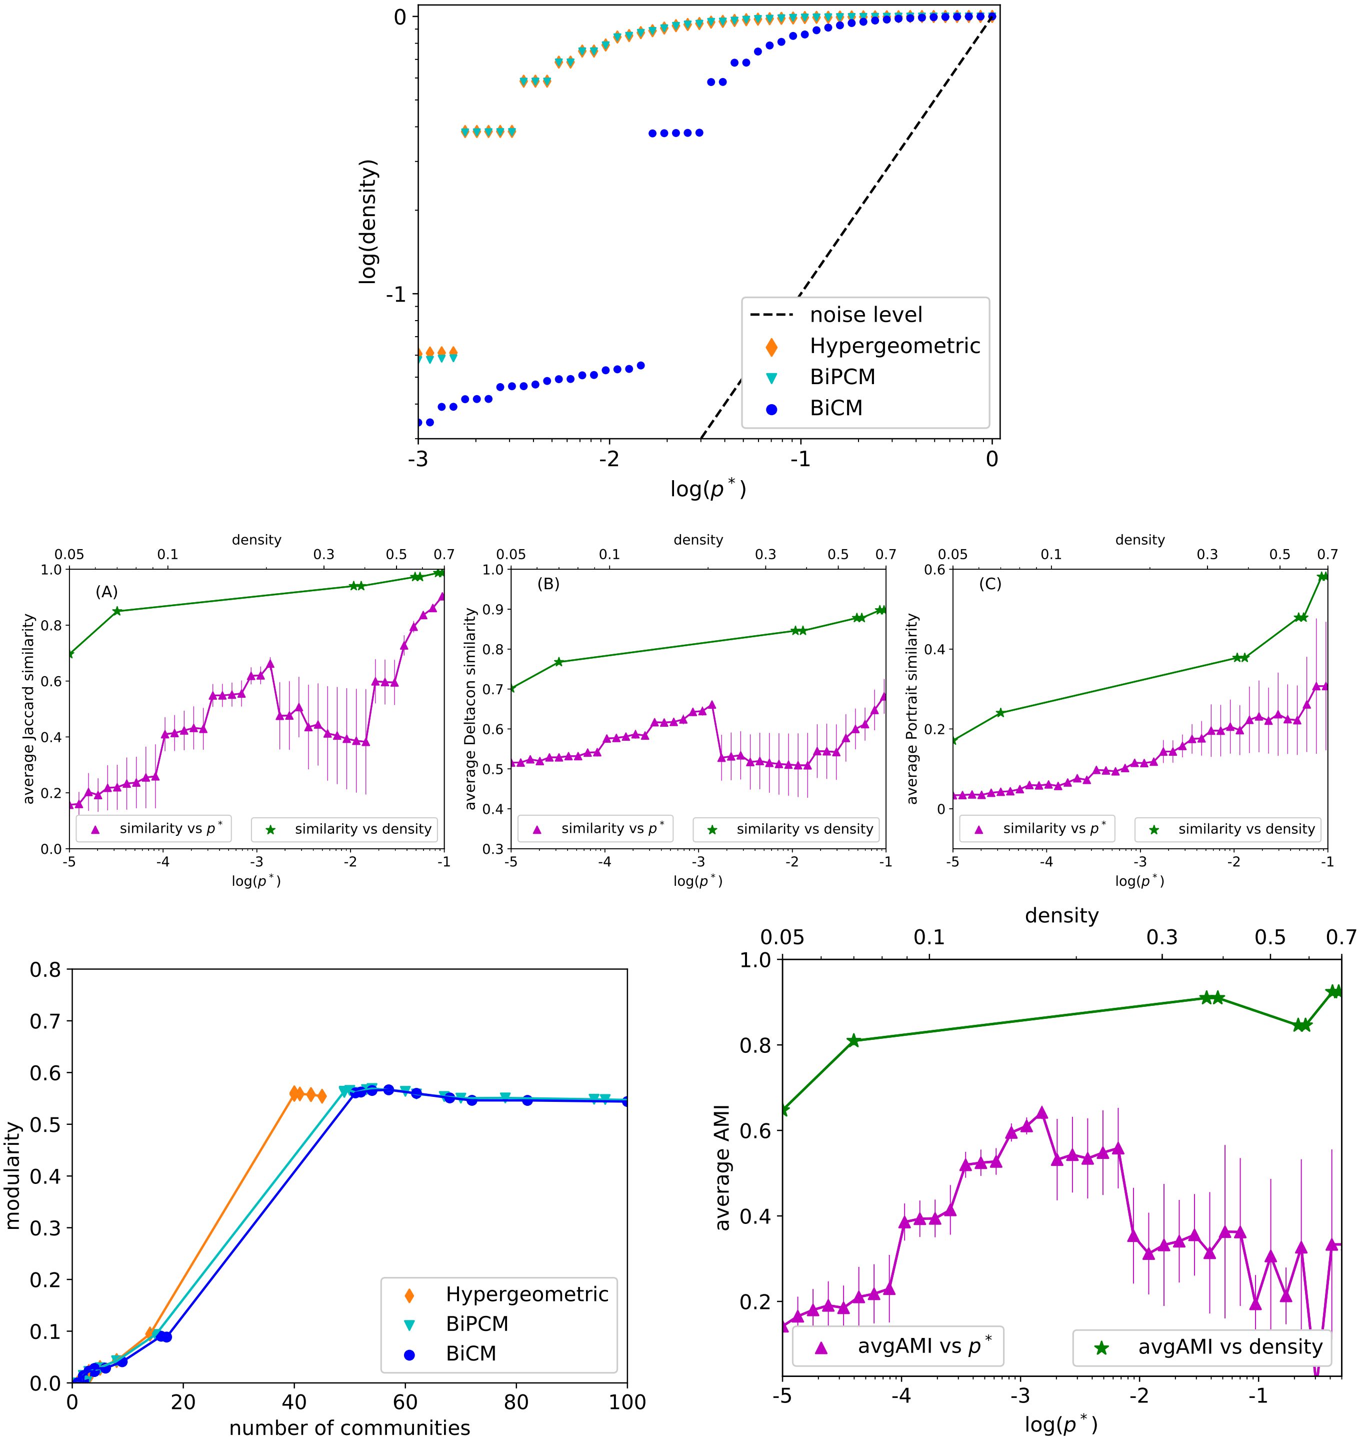


Supplementary Figure 13. *HOST-VIRUS* network. Top panel: density $\rho$ of validated links as a function of $p^*$. Middle panels: (A) Jaccard, (B) DeltaCon, (C) Portrait similarity of validated networks, as a function of either $p^*$ or $\rho$. Bottom panels: (left) Modularity vs number of communities; (right) average AMI for partitions of the validated networks as a function of either $p^*$ or $\rho$. Error bars represent standard deviations over choices of null model pairs.

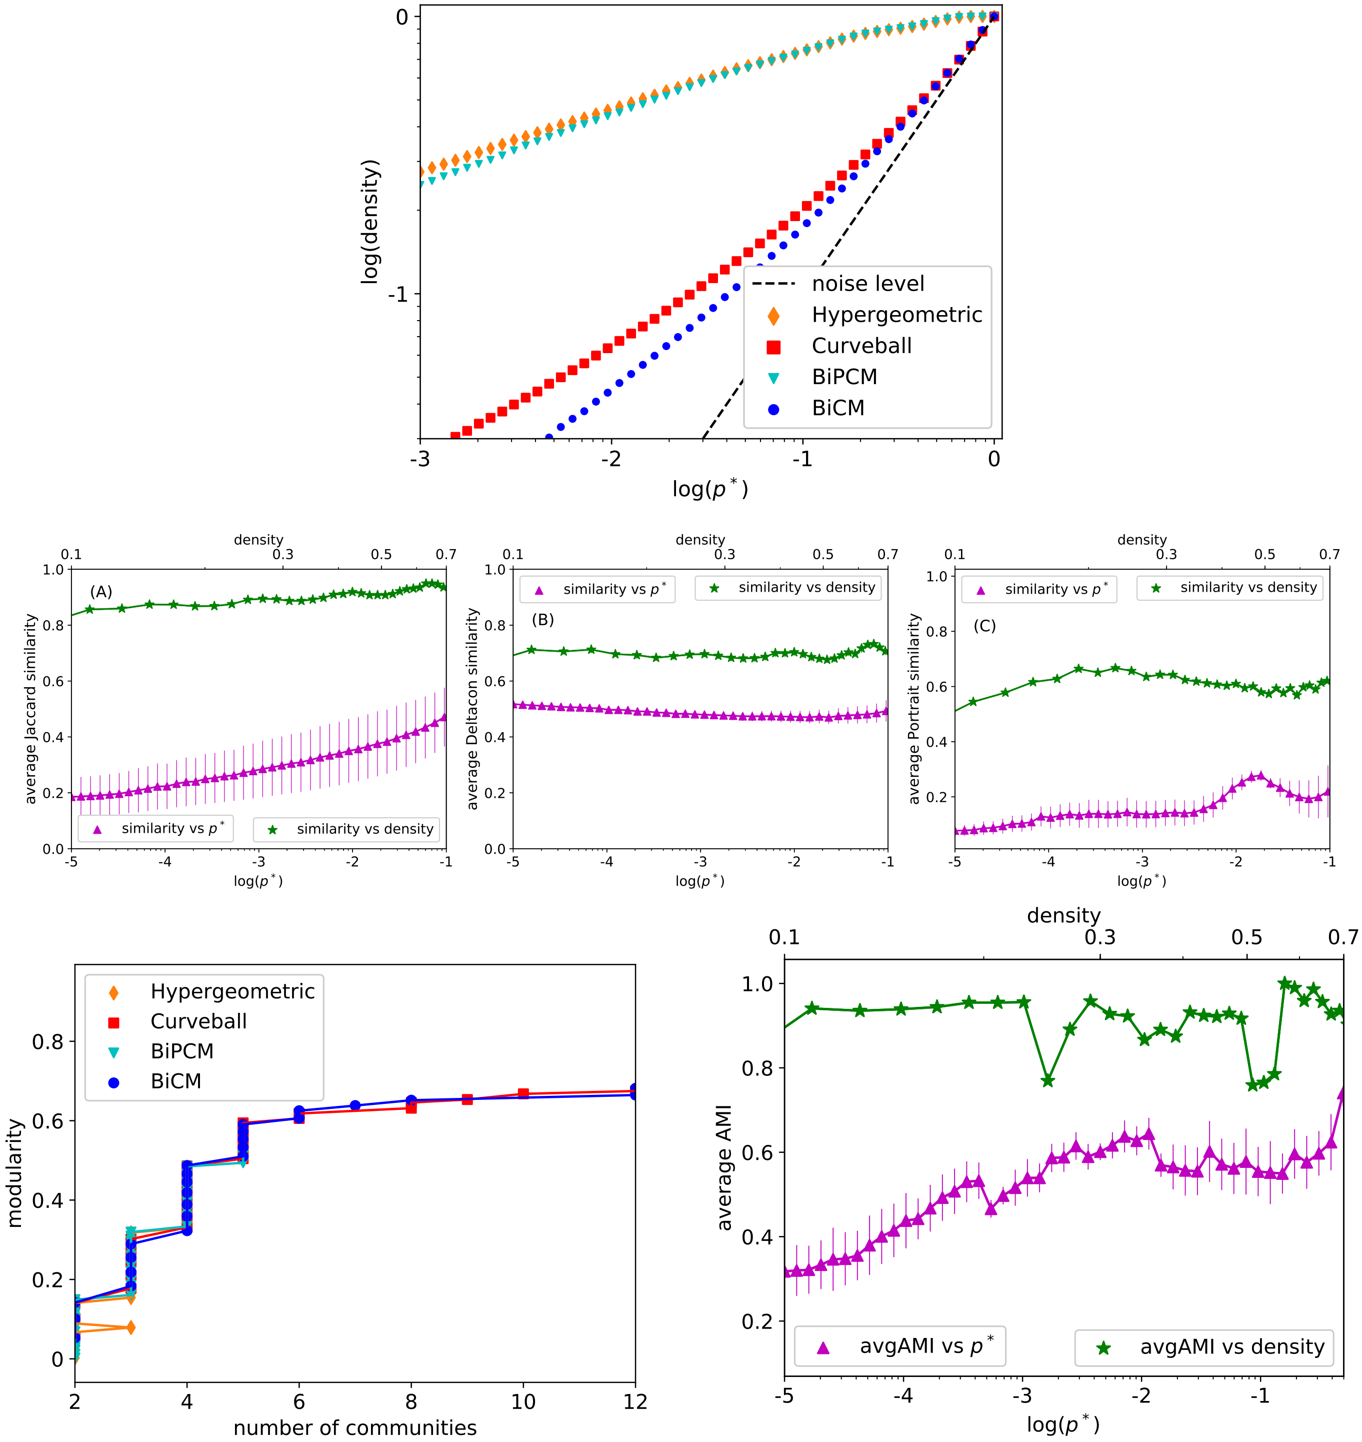


Supplementary Figure 14. *ROBERT* network. Top panel: density $\rho$ of validated links as a function of $p^*$. Middle panels: (A) Jaccard, (B) DeltaCon, (C) Portrait similarity of validated networks, as a function of either $p^*$ or $\rho$. Bottom panels: (left) Modularity vs number of communities; (right) average AMI for partitions of the validated networks as a function of either $p^*$ or $\rho$. Error bars represent standard deviations over choices of null model pairs.

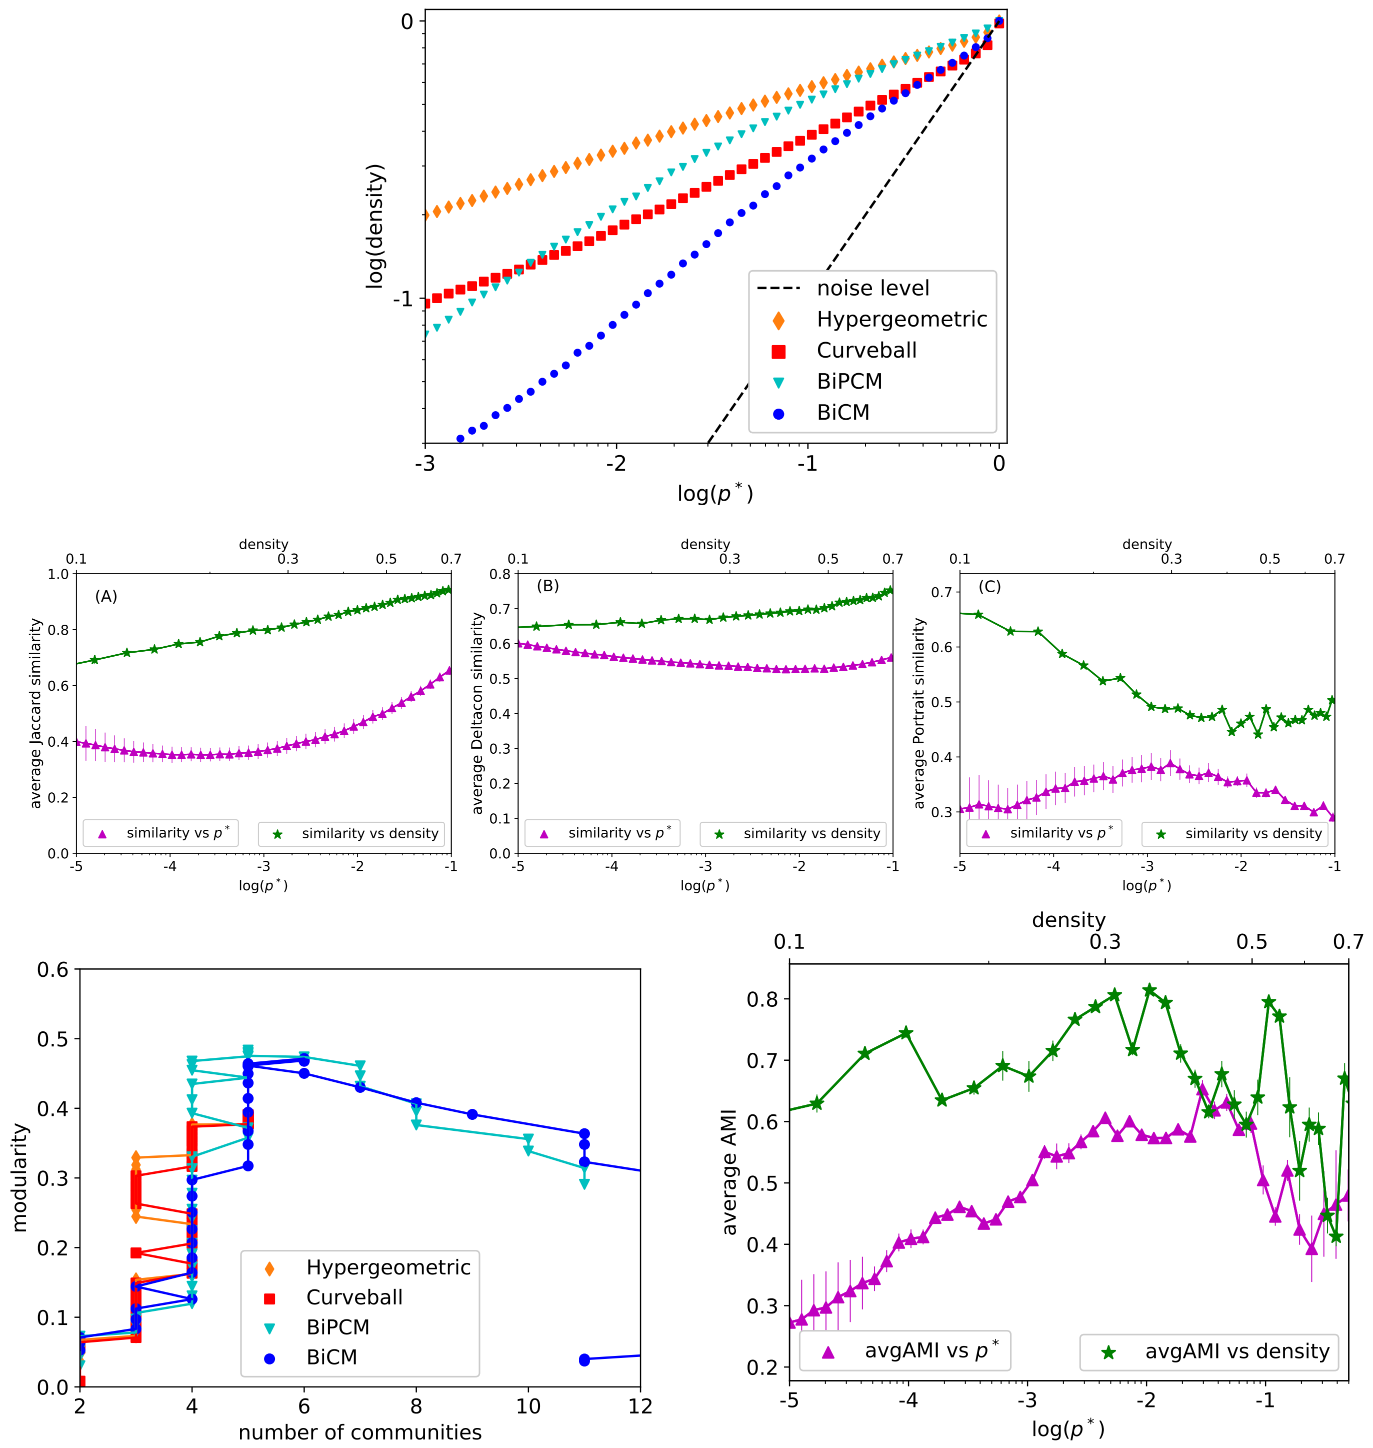


Supplementary Figure 15. *TAYLOR* network. Top panel: density $\rho$ of validated links as a function of $p^*$. Middle panels: (A) Jaccard, (B) DeltaCon, (C) Portrait similarity of validated networks, as a function of either $p^*$ or $\rho$. Bottom panels: (left) Modularity vs number of communities; (right) average AMI for partitions of the validated networks as a function of either $p^*$ or $\rho$. Error bars represent standard deviations over choices of null model pairs.

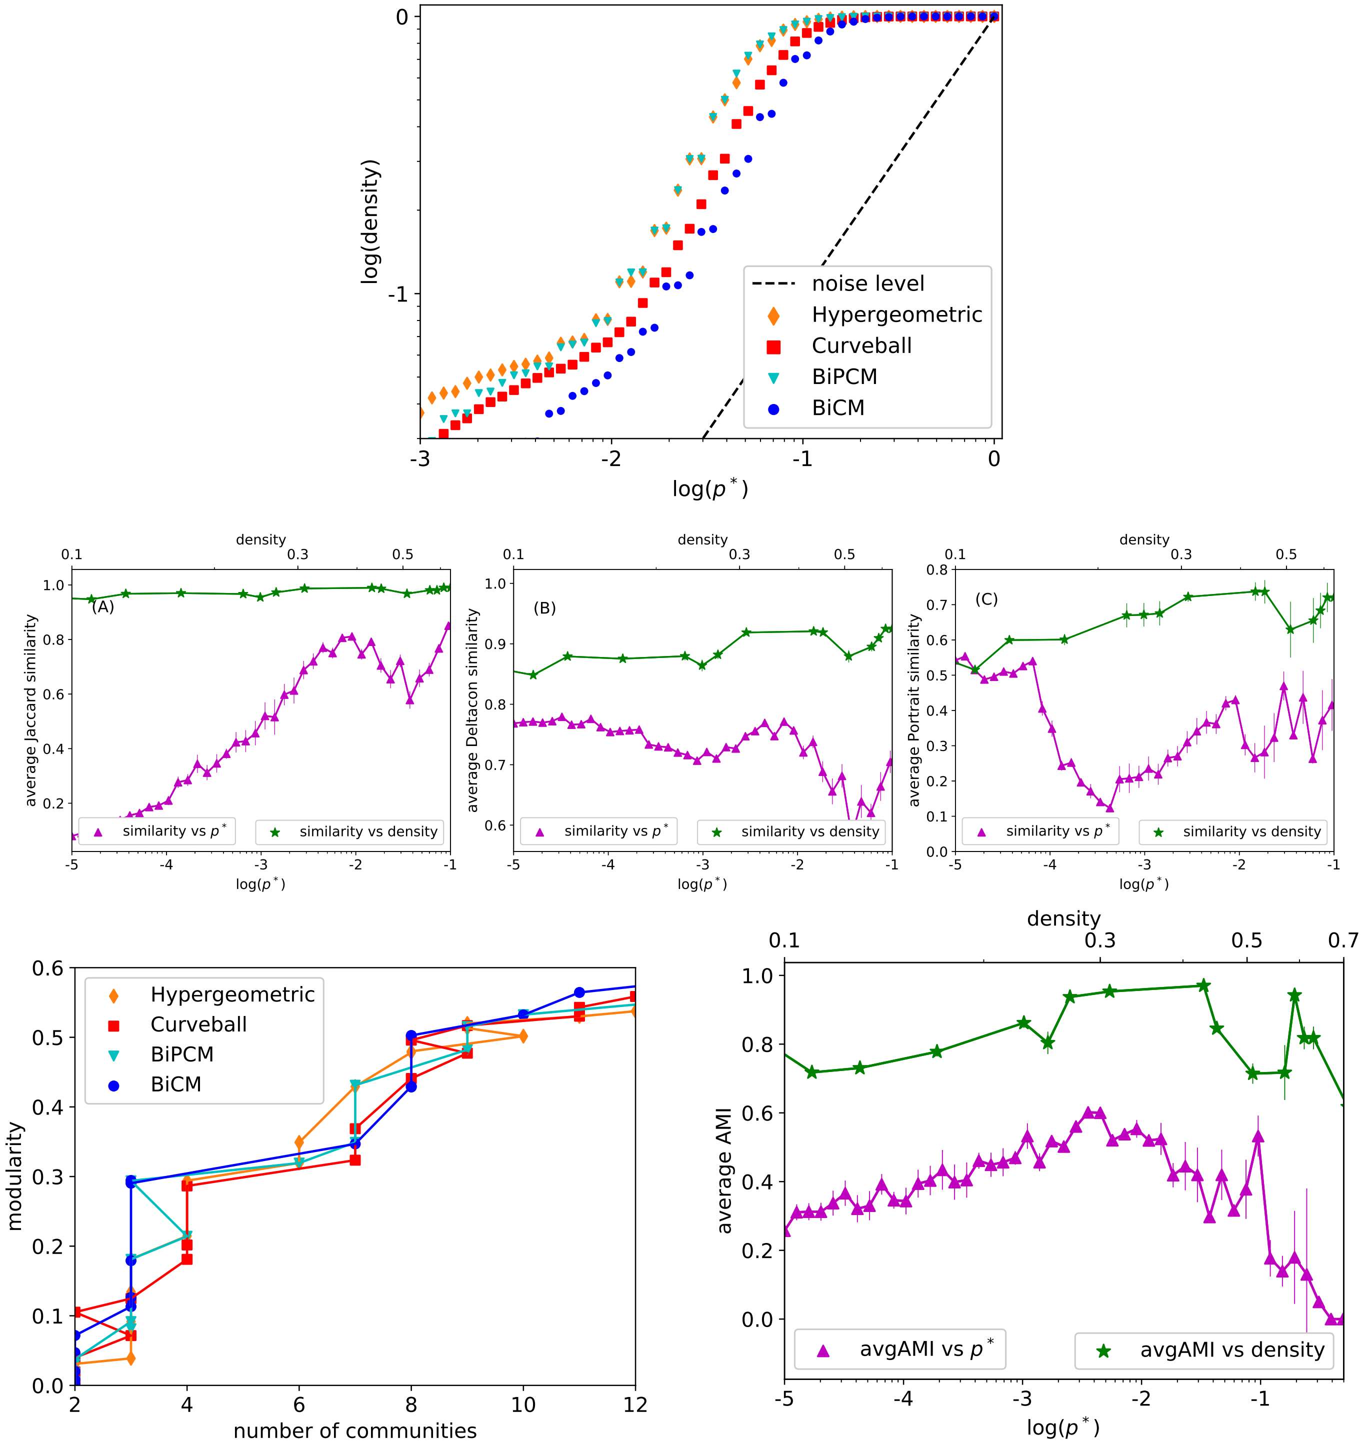


Supplementary Figure 16. *DUTCH* network. Top panel: density $\rho$ of validated links as a function of $p^*$. Middle panels: (A) Jaccard, (B) DeltaCon, (C) Portrait similarity of validated networks, as a function of either $p^*$ or $\rho$. Bottom panels: (left) Modularity vs number of communities; (right) average AMI for partitions of the validated networks as a function of either $p^*$ or $\rho$. Error bars represent standard deviations over choices of null model pairs.

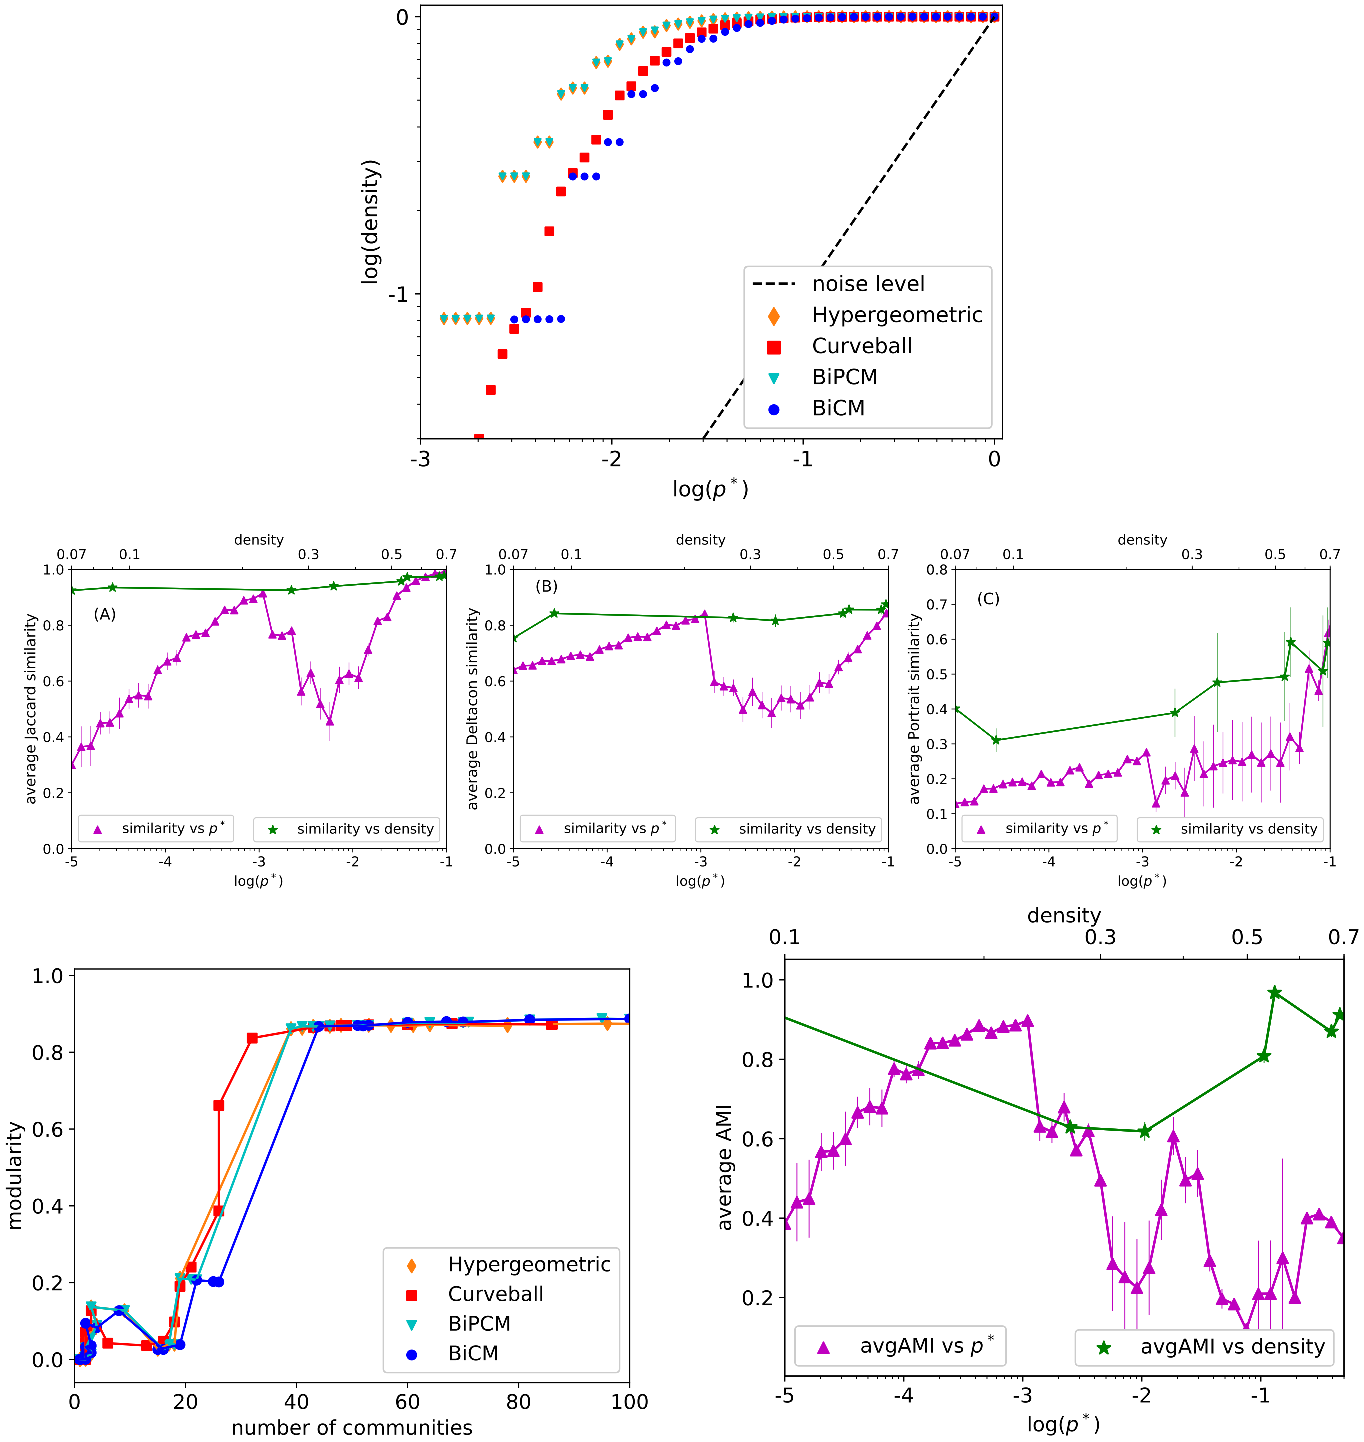


Supplementary Figure 17. *CRIME* network. Top panel: density $\rho$ of validated links as a function of $p^*$. Middle panels: (A) Jaccard, (B) DeltaCon, (C) Portrait similarity of validated networks, as a function of either $p^*$ or $\rho$. Bottom panels: (left) Modularity vs number of communities; (right) average AMI for partitions of the validated networks as a function of either $p^*$ or $\rho$. Error bars represent standard deviations over choices of null model pairs.

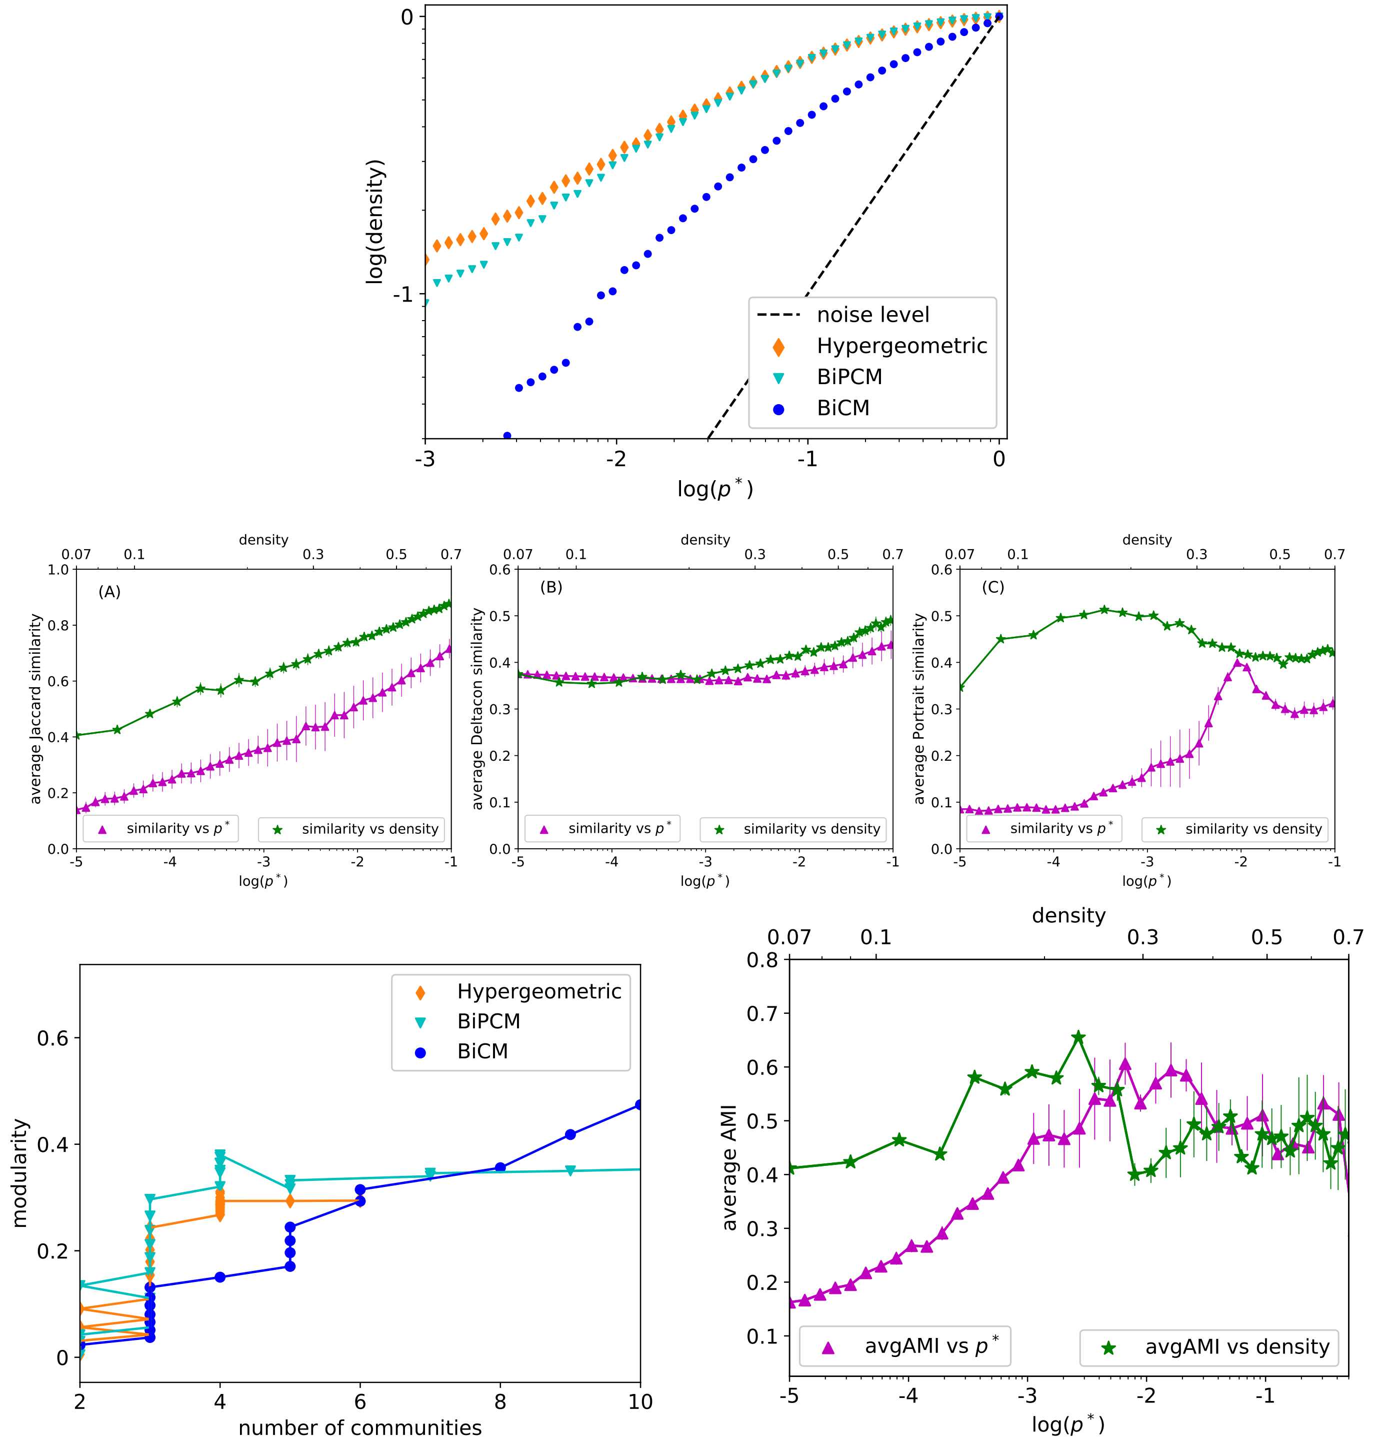


Supplementary Figure 18. *MOVIELENS* network. Top panel: density $\rho$ of validated links as a function of $p^*$. Middle panels: (A) Jaccard, (B) DeltaCon, (C) Portrait similarity of validated networks, as a function of either $p^*$ or $\rho$. Bottom panels: (left) Modularity vs number of communities; (right) average AMI for partitions of the validated networks as a function of either $p^*$ or $\rho$. Error bars represent standard deviations over choices of null model pairs.
